# Supplementary material for: Evaluation of In-Person Counseling Strategies To Develop Physical Activity Chatbot for Women
Source: arXiv:2107.10410 source file (2021-07-22)
Supplement: Supplementary file 1 [file codebook.pdf]

**mPed Codebook**

**HOW TO CODE - INSTRUCTIONs**

In the excel file, you will see 5 columns for each utterance.

Higher-level coding:
**First column** is "domain". You will select the column with a drop-down function and choose the domain of the utterance. Domain refers to the overall topic of conversation, and may not align with the content of each individual utterance.

Lower-level coding:

**Second and Third columns** pertain to intervention "strategies". There are two columns because some utterances may contain more than one intervention strategies. The first strategy coded should be the most significant or relevant to the domain. Strategies refer to the **intention** of the individual utterance.

**Fourth column** is "social exchange". If the utterance contains social exchange, select this column and choose the category.

Fifth column is "task-focused exchange" (excluding the intervention strategies). If the utterance contains task-focused exchange, select this column and choose the category.

All categories must be coded, with no blank spaces left in the coded transcript. For lower-level coding, if none apply, select the option "None". This option should also be selected for phrases included that are not actually spoken by the speakers. Ex) "(affirmative)" or "[laughter]".

Some utterances may contain multiple categories from several of these 5 columns. Here are some examples:
==============================================================

Example 1

Example 2 (Suppose that the overall domain was "Goal")

Mh-hmm. (affirmative)

- ⇨ Choose "Goal" for column 1 (domain), Choose "Agree" for column 4 (social exchange)

As shown above, there is no need to code column 2, 3, or 5.

## COLUMN 1: * INTERVENTION DOMAINS*

### [DOMAIN]

Breakdown of the intervention into the following 14 domains. In this higher-level categorization, physical activity guidelines for adults and older adults should be categorized as "physical activity guidelines", short and long term goal setting as "goal setting". This is to avoid any confusion which may come from similarities of the domains. If the speakers engage in sustained conversation about something not related to the intervention, the entire conversation may be coded as Off-Task. This does not apply if there are only one or two utterances that digress from the overall topic of conversation.

1. Introduction [Introduction] – Generally the beginning of the conversation, when the participant and research staff are greeting each other and no domain has been established. However, the domain of the introduction may have **Strategy1 and Strategy2, or social interactions**
2. Physical activity guidelines [Guideline]
3. Health benefits of physical activity [Benefit]
4. Goal setting [Goal]
5. Self-monitoring/Adherence [Monitoring]
6. Social support for physical activity [Support]
7. Self-efficacy/confidence [Self-efficacy]
8. Motivation [Motivation]
9. Overcoming barriers to being active [Barrier]
10. Relapse prevention [Relapse]
11. Safety of physical activity [Safety]
12. Healthy diet [Diet]
13. Weight loss and maintenance [Weight]
14. Off-Topic Conversations [Off-Task] – Off-Task should also be used for any "wrap-up" or logistic conversation, ie "Ok so next visit will be your randomization visit", etc. When Off-Task is coded as domain, all other columns should be coded as "none"

## COLUMNS 2 & 3: *INTERVENTION STRATEGIES *

### [Strategy1 and Strategy2]

### [Guideline: Physical activity guidelines]

Used when the purpose of the statement is to give general guidelines of physical and aerobic activities for adults. This category includes subcategories such as 1) Key guidelines for aerobic activity – **time spent physically active**, 2) Key guidelines for physical activity – **different types of physical activity**, and 3) Key guidelines for physical activity – **intensity of physical activity.** This strategy should only be used when **the speaker specifically references the guidelines**, and should NOT be used every time the speaker gives general information that could have come from the guidelines. For example, saying "there are many benefits of PA" is NOT a guideline strategy, but saying "guidelines show there are many benefits of PA" IS a guideline strategy.

| Examples: |
|---|

**R:** Today we'll talk about the **current physical activity guidelines** in place for adults.

**R:** The **guidelines recommend** that adults get a minimum of 150 minutes, or 2.5 hours, of moderate to vigorous exercise per week. The goal is at least 300 minutes, or 5 hours.

**R:** It's **recommended** that all adults participate in both aerobic exercise, and muscle strengthening activities. So there are plenty of options for physical activity!

Giving general guidelines of physical and aerobic activities tailored for older adults. This category includes subcategories such as 1) Key guidelines for older adults – **aerobic exercise**, 2) Physical Activity in Older adults – **safety and intensity relative to condition**, 3) Physical Activity and Older adults – **health benefits**, and 4) Physical Activity and older adults – **types of physical activity.**

Examples:

**R:** We recommend that you get at least 150 minutes per week of moderately vigorous physical activity. **Are there any activities you can try that would not hurt your knees?**

**R:** Wonderful. One thing to keep in mind is that in addition to aerobic exercise, current guidelines recommend that **older adults do some balance and muscle training as well**.

**[Benefit: Health benefits of physical activity]**

Used when the purpose of the statement is to identify, emphasize, or ask about health benefits such as **1) Lower risk of all-cause mortality, 2) Cardiorespiratory health: health of the lungs, heart, and blood vessels**, **3) Cardiometabolic health**: A term that encompasses cardiovascular diseases and metabolic diseases, such as type 2 diabetes. Cardiovascular disease and metabolic disease share a number of risk factors, and reducing risk of one can reduce risk for the other. Cardiometabolic health and weight status are also closely related issues and are often considered together, **4) Bone and muscular health**: Healthy bones, joints, and muscles are critical to the ability to do daily activities without physical limitations such as climbing stairs, working in the garden, or carrying a small child, **5) Functional Ability and Fall Prevention**: Physical function, or functional ability, is the capacity of a person to perform tasks or behaviors that enable him or her to carry out everyday activities, such as climbing stairs, or to fulfill basic life roles, such as personal care, grocery shopping, or playing with grandchildren. Loss of functional ability is referred to as functional limitation.

Examples:

**R:** Guidelines suggest that **physical activity reduces risk** of heart disease, stroke, diabetes, and high blood pressure. But it also increases mood, energy, self-confidence, and even cognition.

**R:** Absolutely, even though the effects aren't immediately visible, getting more physically active is an **excellent way to protect your health** in that regard. Keep up the good work!

**R:** That's so great that you're already sleeping better at night!

**[Goal: Goal Setting]**

Used when the purpose of the statement is to introduce, encourage, or ask about short-term goals. NOTE. the short term goals (e.g., step counts per day) are subject to change based on participants' baseline scores. This category includes 1) Short-term goal setting: **safety and gradual increases** and 2) Short-term goal setting: **realistic and achievable** goals.

Examples:
**R:** This is your week one hour steps **per day** that we would like you to meet.

**R: Each week, we want you to increase your daily step count goal by 20%**. So, if your baseline is 3,500 steps per day, your short-term goal for week one is to walk 4,200 steps per day.

**R:** A weight loss goal of 1-2 pounds **per week** over the next 6 weeks would be a great place to start. You can achieve this by reducing your caloric intake to 1500 calories per day.

**R:** Do you think you can start out by walking just 10 minutes more each day?

Used when the purpose of the statement is to introduce, encourage, or ask about long-term goals. Long term goals address the final goal that the participant hopes to reach and maintain. To differentiate with short-term goal setting, it is important to check whether the researcher mentions "**long-term goals**". This category includes 1) Long-term goal setting: **making a plan for success** and 2) Long-term goal setting: **framing large goals in smaller increments**.

Examples:
**R:** Your **long-term goal** is to maintain ten thousand steps per day as best as possible.

**R: Your long term goal is** to reach 10,000 steps per day. Of course, this won't happen overnight. Since it is a long term goal, the hope is that you will eventually reach it and then most importantly, be able to maintain it.

**R:** Let's start with the goal itself. A good **long term goal** is to lose 10% of your total body weight over the next six months. For you, that means losing 23 pounds.

**R:** Eventually, we want you to be able to jog for one mile without pausing.

**[Monitoring: Self-monitoring and adherence]**

Self-monitoring informs participants to be encouraged to take accountability for their goals, and to stick to the plans that they have made with minimal external intervention. This category should be used whenever a statement is meant to encourage, express or assess 1) **self-accountability and visual reminders**, 2) **measuring intensity** of physical activity, and 3) **tracking** physical activity.

| Examples: |
| --- |
| **R:** Me too. Today I want to talk to you about **how to keep on track for your goals, even when you go a while without hearing from me.** |
| **R:** That sounds good, too. I think if you do both of those things you should have an easier time **remembering to take your medication**, and then you can focus on your other goals. |
| **R:** You could also try **monitoring** your heart rate. Using two fingers on the outer part of the inside of your wrist, count the number of heart beats in 30 seconds, and multiply that by two to get your resting heart rate. Your heart rate should increase during exercise. |
| **R:** Have you been getting out for regular exercise? |
| **R:** Have you been remembering to take your medication regularly? |
| **R:** Remember that you should be getting moderate-to-vigorous exercise, not just going for leisurely walks. |
| P: I think I need something to hold me accountable, I keep forgetting. |

**[Support: Social support for physical activity]**

Informing about social support. Social support can come in various forms. Some options are having others that you can talk to about your goals and who can keep you accountable, or having friends and family who you can ask to participate directly in your goals. This category includes informing participants, encouraging them to acquire, or asking them about 1) **PART, how to involve family in physical activity** and 2) using **physical activity for quality time with important people**.

| |
| --- |
| **R:** I'm glad to hear it. The first thing I want to talk about today is **social support.** The people around you can be a really important part of motivating you to be physically active. |
| **R**: It is important to have people around you that can motivate you to increase physical activity. What **social support** do you have in place now? |
| **R**: **Asking people to join you** in increasing physical activity can seem daunting, but many people might have similar goals and not know how to get motivated. So they may receive it very well. |
| **R:** Even just talking to the people around you about your goals is a fantastic first step, but it |

can also help to get them directly involved. How do you think you could involve your family members in your goals?

**R:** Have you been going for walks with your husband lately?

**[Self-efficacy: Self-efficacy/confidence]**

Self-efficacy is defined as the belief in one's own ability to achieve actions necessary to produce a desired effect. In more detail:

Bandura's self-efficacy theory suggests **four main sources of influence in the development of self-efficacy**: past performance, vicarious experiences (observing others perform), verbal persuasion, and physiological cues.

**1)** ***Past performance*** **is considered the most powerful method of developing self-efficacy.** For example, a client who mastered performance on one machine such as the bicycle has self-efficacy related to that task. This efficacy based on past performance can be used to instill efficacy on other tasks such as on the elliptical machine. Success breeds success.

**2)** ***Vicarious experiences*** **or observing others perform** also is effective. If a client has seen someone else walk a mile, she may feel more confident in her own ability to walk a mile.

**3)** ***Social persuasion*** involves encouragement from others. Coaching and giving evaluative feedback on performance are common techniques. An example would include praising a client for taking four walks for the past week, giving him a few tips on how to work walking into his busy schedule and expressing confidence that he can reach his goal of walking five times per week next week.

**4)** **Experiencing physiological cues** such as anxiety and stress when thinking about exercising at a gym or participating in a team sport can negatively impact self-efficacy, but this is less influential than the other sources. Helping a client learn how to maintain an optimal level of physiological intensity for performing the task through relaxation techniques and self-talk can increase efficacy.

This category includes utterances that help participants develop positive thoughts and feelings (such as confidence) related to physical activity, as well as participant expressions about their own self-efficacy or doubt in their abilities.. More specifically, this category includes 1) maintenance of health behaviors over time, 2) confidence in ability and willingness to try new things, 3) not giving up easily and staying motivated.

**R:** I can see why that would be daunting. But look at the progress you have already made! If you stick to each short-term goal, I think you'll be surprised by just how **capable** you really are.

**R:** I can see why that would be intimidating. The good news is that physical activity can be **incredibly simple.**

**R:** I can see why that might be frustrating. Keep in mind all of the work you've put into identifying your barriers and creating strategies for overcoming them and staying motivated. Sometimes this is the hardest part, and it's something you never tried before. **You've already**

**made such progress!**

**R:** That's awesome. You should be really proud of yourself.

**P:** That's going to be really difficult... I'm not sure I'll be able to manage it.

**[Motivation: Motivation]**

Statements meant to motivate the participant or inform how to stay motivated, as well as participant statements expressing motivation or lack thereof. This category addresses situations such as 1) getting bored with a routine, 2) getting back on track after failures, and 3) trying new activities to re-motivate oneself.

Motivation refers to Intrinsic OR Extrinsic motivation. ***Intrinsic motivation*** is defined as doing an activity because of its inherent satisfactions. When intrinsically motivated the person experiences feelings of enjoyment, the exercise of their skills, personal accomplishment, health benefits and excitement.

***Extrinsic motivation*** refers to doing an activity for instrumental reasons, or to obtain some outcome separable from the activity *per se*. For example, when a person engages in an activity to gain a tangible or social reward or to avoid disapproval, they are extrinsically motivated. SDT, however, conceptualizes qualitatively different types of extrinsic motivation, that themselves differ in terms of their relative autonomy.

**R:** Great! Well today we are going to talk about how to **stay motivated** over time, and what to do if you start to lose motivation.

**R:** For example, if your goal is to walk every day, but you get bored of walking the same route, **are there new places you can try walking?**

**R:** The best way to combat that is to identify some ways that you can get back on track and **re-motivate** yourself.

**R:** It sounds like you might be able to stay more motivated if you shake up your routine a little bit. Have you considered **trying a new activity** such as dancing, or playing tennis?

**P:** I started going to these Zumba classes, they've been super fun!

**R:** Keep up the good work!

**[Barrier: Overcoming barriers to being active]**

Informing how to identify & overcome barriers, or participants identifying and talking about their barriers. This category includes 1) identifying barriers and lack of time, 2) lack of motivation and neighborhood safety, and 3) environmental safety and weather.

**R:** Some common goals are lack of time, lack of motivation, and concerns for safety. Can you identify what your **own barriers** are?

**R:** I see. So family obligation can be a **barrier** for you as well?

**R:** That makes sense. **Identifying your barriers** ahead of time allows you to make a strategy for combating them, which can help with long-term success

**R:** Absolutely, I can see why that might be challenging. Sometimes when environmental concerns like neighborhood safety or the weather are a factor, it can be useful to find a reliable way to get physical activity inside.

**R:** Has it been any easier lately to fit some physical activity in to your schedule?

**P:** My brother passed away last month... I've been so depressed.

**[Relapse: Relapse prevention]**

Informing the importance of strategies to avoid relapsing once they have established new, healthier habits. Also any time a participant talks about relapsing. Asking participants to identify the factors that cause them to relapse, or go back to their old, unhealthy habits. This category includes 1) relapse prevention: eliminating triggers and social support and 2) relapse prevention: guilt.

**R:** That can definitely be challenging. What is causing you to **relapse** into old habits?

**R:** It sounds like the best thing to help you **stay on track** would be to eliminate that temptation. How do you think you can do this?

**R:** It's important to keep in mind that you don't have to give up everything completely. And if you get off track, its okay!

**P:** I was doing so well until my husband started buying junk food again.

**[Safety: Safety of physical activity]**

Statements meant to inform participants about the importance of safety during physical activity, or meant to ensure safety. Also participant comments about safety. This includes 1) Safety: environmental safety, safety for walking at night, 2) Safety: staying hydrated, stretching, and 3) Safety: physical exercise with previous conditions and pain.

**R:** That's a great point. It's very important to keep safety in mind while being physically

active. What else do you think you can do to stay **safe while exercising**?

**R:** Additionally, I know you mentioned that you don't walk much at night, but if you do, be sure to **wear reflective clothing or a light.**

**R:** That is a great place to start. And then once you begin to feel stronger, you can increase the length of your walks, and even begin to add more moderate or vigorous activity.

**P:** I hate walking at night because I feel like cars can't see me.

**[Diet: Healthy diet]**

Informing & emphasizing the importance of 1) Breakfasts, 2) Small and balanced meals, 3) management of overweight and obesity, and 4) weight loss in relation to regular physical activity.

**R:** I see. It's important to choose **breakfast foods** that fill you up and give you long lasting energy. Waiting until you want to eat is fine, but do you think there is a healthier option you can choose?

**R:** It sounds like you could benefit from breaking that cycle. **Try eating a little bit more in the morning so that you stay fuller for longer, and then eating as soon as you get hungry.** In general, you want to stay between a three and a six on the hunger scale.

**[Weight: Weight loss and maintenance]**

**R:** So today we want to talk about healthy **weight management**. The first step to understanding weight management, is understanding what it means to be overweight or obese.

**R:** In order to lose weight, you have to be in a **calorie deficit**. While regular physical activity can help with that, it will also likely require you to reduce your **caloric intake** as well.

**Part 1. Social Exchange**

**Personal Remarks, Social Conversation**

Greetings, initiating contact through friendly statements that are part of a formal greeting, return of friendly gestures and greetings, and goodbyes.

**Greeting –** Should only be used when a formal greeting such as "Hi, Hello, or Good Morning" is used.

| |
|---|
| Example:<br>***R:*** *Hello, how are you doing?* |

**Goodbye**

| |
|---|
| Example:<br>*Bye.*<br>*I hope that you have a wonderful day.*<br>*Have a wonderful day.*<br>*Have a great evening!*<br>*It was nice to chat with you.*<br>*Good luck (when said at the end).* |

**Approve/Encourage: Shows Approval- Positive responses**

**Compliments, expressions of approval, encouragement, gratitude, praise, reward, respect or admiration directed to the other person present. Includes such statements as "Thank you," "You're welcome."**

| |
|---|
| **Examples:**<br>*That was terrific! [re. something the other has done]*<br>*I really appreciate what you've done.*<br>*Thank you.*<br>*You're welcome* |

**Disapprove/Discourage: Shows Disapproval – Negative responses**

**Any indication of disapproval, discouragement, criticism, denial, complaint, rejection, coolness or disbelief directed expressly to the other person present. This includes statements that contradict or refute something said by the other, or imply disagreement with or rejection of the other's hypotheses, ideas or opinions.**

**This could also include expressions of doubt or uncertainty.**

| |
|---|
| **Examples:**<br>*No, I don't think so.*<br>*Two pounds. That's not good enough*<br>*I guess I could try… but that is going to be really difficult.*<br>*I'm not sure that's going to be possible…* |

**Agree: Shows Agreement or Understanding (Agree)**

Included in this category are **signs of agreement or understanding**, including approval of previous utterances by the other party. This category also includes indicators of **sustained interest, attentive listening or encouragement** emitted by either party when he or she does not hold the speaking floor (called **"Back-Channel Responses"**).

| |
|---|
| Examples: |

*I see.*
*Yes, that's right.*
*I know.*
*Okay.*
*Oh, really.*
*You were right.*
*Me neither.*
*I absolutely understand.*
*No problem.*
*That's a good idea.*
*That sounds good.*
*Yes, I can do that.*
*I can see why you feel that way.*
*Finding time for physical activity can definitely be difficult. (confirmation, in response to participant suggesting this)*

**Back-Channel Responses**
*Mmm-huh.*
*Yeah [I'm listening]…*
*Right [go on…]…*

**Incomplete: Incomplete**

Incomplete utterances. Only grammatically incomplete utterances should be coded as such. Long conversations consisting of fragmented sentences which do not have clear meaning should not be coded, and should be highlighted instead. Sentences that get cut off, but which are grammatically sound and carry meaning, should not be coded as incomplete and should instead be coded normally. For example, "Yeah, that would be difficult but… " "… I think I can try anyway".

Examples:
*Umm, it will defi-...*
*Umm…*
*..Well… If.*

**Part 2. Task-Focused Exchange**

**Orient: Gives Orientation, Instructions (Orient)**

Introductory statements **tell the other person what is about to happen, what is expected during the intervention, or serve to orient the other to the major topics of discussion.** The purpose of these statements is to guide the other person in terms of what to expect during the intervention.

Examples:
*This is the Physical Activity Intervention Presentation with participant thirteen nineteen. [00:00:05.640] I'm RA twenty-three and it is March 10th, 2014.*

| |
|---|
| *Umm, our study is twelve months long, umm, and what it is we're comparing pedometer and mobile phone-based physical activity programs to see if that does motivate you to become more physically active.* |

**Information exchange**

**Ask-GenInfo: Asking for general (non-personal) information**

Asking about (non-personal) information.

| |
|---|
| Examples:<br>*what do you mean by family obligations?*<br><br>*Could you give me some examples of healthy snacks?* |

**Give-GenInfo: Providing general (non-personal) information**

Providing (non-personal) information.

| |
|---|
| Examples:<br>*So generally, ten minutes of walking is about a thousand to a thousand and two hundred steps.*<br><br>*In the app, you can log down your activities that you do even if you're not wearing the pedometer.*<br><br>*Your goal is to walk 5,000 steps per day this week.* |

**Ask-PerInfo: Asking for personal information**

Ask about the conversational partner's information. This could include factual information regarding personal experience, living environment, and work-related utterances.

| |
|---|
| Examples:<br>*How is your neighborhood?*<br>*What social support do you have in your life?*<br>*Where do you like to go for exercise?*<br>*What are your greatest barriers to physical activity?* |

**Give-PerInfo: Self-disclosure of personal information**

Self-disclosure of one's information. This could include factual information regarding personal experience, living environment, and work-related utterances. This can also include statements about a person's emotional state.

| |
|---|
| Examples:<br>*The closest gym is on Sixteenth Street.*<br>*I work 40 hours a week.* |

| |
|---|
| *My family is very supportive of me.*<br>*I'm mostly afraid to go outside alone at night*<br>*I've been really excited to get started.* |

**Check-Understanding: Asks for Understanding**

Check with the other to see if information that was just said has been followed or understood (i.e., in essence asking, "Do you understand what I'm saying?").

| |
|---|
| Examples:<br>*Do you follow?*<br>*Do you understand?*<br>*Do you have any questions for me?* |

**Ask-Repeat: Bid for Repetition**

Requesting repetition of the other's previous statement. In other words, asking for the same information again.

| |
|---|
| Examples:<br>*I did not understand that question.*<br>*Could you explain that again?*<br>*Per day?*<br>*Oh, really?* |

**Ask-Opinion: Asks for Opinion**

Questions that ask for the other **person's opinion, point of view or perspective.** Includes questions that invite the other person 's judgment, or ask for preferences, expectations, or survey of the problem.

| |
|---|
| Examples:<br>*What do you think could have caused this?*<br>*What do you think would help?*<br>*Do you think you could achieve this amount per week?*<br>*What do you think you can do to increase the social support you have?*<br>*How do you think you can overcome this barrier?*<br>***Note: Asking a participant to identify their barriers is asking for personal information, whereas asking how they think they can overcome those barriers is asking for an opinion. In the former, they are being asked to identify personal information, whereas in the latter they are being asked their opinion about how to fix it.* |

**Give-Opinion: Opinion response**

Indication of one's "opinions" in response to the partner's statement. **Opinion responses should be highly subjective and include one's judgments. Usually, they may contain "I think" and "I feel" statements. Can also refer to one's opinion of the other's actions, often which will be coded socially as approval.**

Examples:
*I think I can do that.*
*That sounds reasonable.*
*I think things would be easier if I scheduled exercise ahead of time.*
*I think its great that you're getting your family involved.*
*I'm happy to see that you're reaching your goals*
***Note: Similar to above. A participant stating that "not having a routine is a barrier to exercise" is giving personal information, whereas the above statement is an opinion about how they think they could fix it.*
